# Supplementary material for: Model-Based Iterative Reconstruction of Three-Dimensional Magnetisation in a Nanowire Structure Using Electron Holographic Vector Field Tomography
Source: arXiv:2411.15323 ancillary file (2025-05-02)
Supplement: Supplementary file 1 [file Supplementary_material.pdf]

# Model-Based Iterative Reconstruction of Three-Dimensional Magnetisation in a Nanowire Structure Using Electron Holographic Vector Field Tomography

## Supplementary Material

22/02/2025

Aurys Šilinga[1], András Kovács[2], Stephen McVitie[1], Rafal E. Dunin-Borkowski[2], Kayla Fallon[1] and Trevor P. Almeida[1]

1. *School of Physics and Astronomy, University of Glasgow, Kelvin Building, Glasgow G12 8QQ, Scotland, United Kingdom*
2. *Ernst Ruska-Centre for Microscopy and Spectroscopy with Electrons, Forschungszentrum Jülich GmbH, Wilhelm-Johnen-Straße, 52428 Jülich, Germany*

## S1. Reconstruction of simulated uniformly-magnetised nanowires

Simulations have previously been used to assess how the range of sample tilt angles, sample tilt increment and sample orientation can affect three-dimensional (3D) reconstruction of magnetisation $\vec{\boldsymbol{M}}$ [1]. It was found that a magnetic vortex state can be reconstructed with an average error of below 1 % from two orthogonal tilt series with ranges of ±60°, regardless of its orientation. The sample described in the main text, which contains a magnetic vortex state and uniformly-magnetised regions, was imaged using two tilt series with a 10° tilt increment and tilt ranges of -60° to 30° and -60° to 0°.

In order to assess the reconstruction errors in uniformly-magnetised parts of the sample, 400-nm-long, 50 nm x 50 nm square-cross-section nanowires were simulated with different magnetisation directions. In the simulations described below, a 0° tilt orientation corresponds to the electron beam passing along the *z*-axis and $\mu_0|\vec{\boldsymbol{M}}|$ is taken to be 1 T for simplicity. It is initially assumed that the geometrical model of the sample is not affected by missing wedge errors, which are discussed later in this section.

Fig. S1a shows simulations of a nanowire magnetised along the *x*-axis, for which a phase measurement at 0° would yield the result shown in Fig. S1b. For the same angular spacing and tilt ranges as in the experiment described in the main text, Fig. S1c shows that the distribution of $\vec{\boldsymbol{M}}$ determined using model-based iterative reconstruction (MBIR) has an error of below 3 % in most of the volume of the nanowire, apart from a small number of voxels at the corners. The average error in the magnitude of $\vec{\boldsymbol{M}}$ in the nanowire cross-section, which is shown in Fig. S1d, is below 1%. If the magnetisation direction is instead oriented along the *y*-axis, as shown in Fig. S2a, then a smaller total phase shift is detected, as shown in Fig. 2b. Fig. S2c shows that the errors in the magnitude of $\vec{\boldsymbol{M}}$ determined using MBIR are again greatest at the sample corners, while Fig. S2d shows that the average error in the cross-section is again below 1%. If the magnetisation direction is instead oriented along the *z*-axis, as shown in Fig. S3a, then no magnetic phase shift is detected at 0°, as shown in Fig. S3b. Fig. S3c shows that the errors are again greatest at the sample corners, while Fig. S3d shows that the average error in the cross-section is again below 1%.

The simulations show that, for the same imaging orientations as in the experiment, the average error in the magnitude of $\vec{M}$ in the reconstructions is below 1%. Reconstruction errors close to the nanowire surface likely arise because of the limited and asymmetrical tilt range, as well as the range of possible configurations of $\vec{M}$ and the effects of digitisation (*i.e.*, finite pixel size). Although MBIR finds a distribution of $\vec{M}$ that minimises the error between the simulated and input phase images, different configurations of $\vec{M}$ can produce equivalent phase images, in particular when the tilt ranges are limited. In the present sample, voxels at the corners of the geometrical model are the least constrained and show the greatest errors.

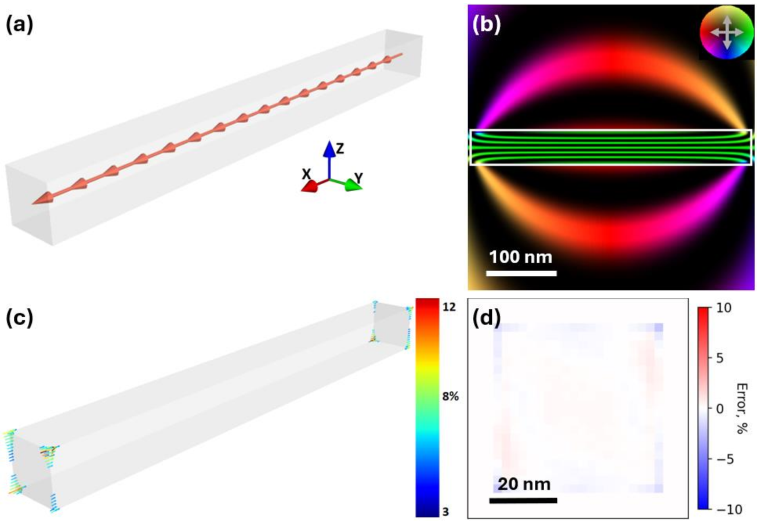


***Fig. S1. Reconstruction of a simulated nanowire magnetised along the x-axis.*** *(a) Model of a 400-nm-long, 50 nm x 50 nm nanowire, showing the sample geometry and the* $\vec{M}$ *direction. (b) Phase contour map at 0° tilt, coloured to show the direction of the projected in-plane* $\vec{B}$ *field (inset), displayed as* $\cos(12\varphi_{mag})$*. The sample outline is marked in white. (c) Reconstruction with the* $\vec{M}$ *vectors scaled and coloured to show the magnitudes of errors greater than 3%. (d) Average* $\vec{M}$ *magnitude error in a cross-section, demonstrating over and under estimates of below 1%. The greatest errors are at the corners of the nanowire, where the separation of* $\vec{M}$ *and* $\vec{H}$ *is ambiguous. See text for details.*

The geometrical model of the sample affects the reconstruction because it defines where in space the magnetic material can be located. If the geometrical model of the square-cross-section nanowire in Fig. S4a were to be generated from experimental electron holograms without accurate missing wedge correction, then the geometrical model would typically be larger than the true nanowire. It was observed that FEBID nanowire edges can appear diffuse when imaged experimentally due to uneven surface texture and variations in material composition. This blurring typically results in a ~5 nm error when determining the position of the sample surface and limits the precision of any missing wedge correction. Accordingly, a 5 nm error was introduced when correcting for the missing wedge in the following simulation. Fig. S4b shows a cross-section of a partially-corrected model generated for the same imaging orientations as in the main text. As the model incorrectly describes some of the vacuum as magnetic material, the reconstructed distribution of $\vec{M}$ has errors close to some of the sample surfaces. Fig. S4c shows that the values of $\vec{M}$ are then spread out, although the peak corresponds to the correct value for the material. The spread is attributed to the intermixing of vacuum and material values. Fig. S4d shows the average error in the cross-section, which is influenced by an overestimation of the

vacuum values and a reduction of the values in the nearby material. The reconstructed distribution has a mean value of $\mu_0|\vec{M}|$ of 0.92 T and a standard deviation of 0.14 T. The results show that, if surface errors are present, then the reconstruction of a uniform magnetic domain can produce a distribution of values of $\vec{M}$, albeit one in which the peak is close to the true value.

Taken together, the simulations show that a uniformly-magnetised nanowire can be reconstructed with an average error of below 1% for the imaging orientations used in the main text. However, errors in the geometrical model of the nanowire can cause vacuum and material values to intermix close to the surface.

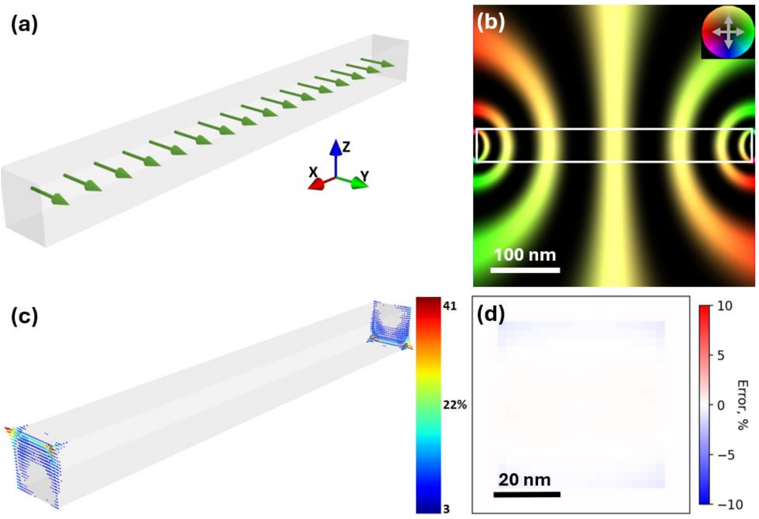


***Fig. S2. Reconstruction of a simulated nanowire magnetised along the y-axis.*** *(a) Model of a 400-nm-long, 50 nm x 50 nm nanowire, showing the sample geometry and the* $\vec{M}$ *direction. (b) Phase contour map at 0° tilt, coloured to show the direction of the projected in-plane* $\vec{B}$ *field (inset), displayed as* $cos(12\varphi_{mag})$ *The sample outline is marked in white. (c) Reconstruction with the* $\vec{M}$ *vectors scaled and coloured to show the magnitudes of errors greater than 3%. (d) Average* $\vec{M}$ *magnitude error in a cross-section, demonstrating over and under estimates of below 1%. The greatest errors are at the corners of the nanowire, where the separation of* $\vec{M}$ *and* $\vec{H}$ *is ambiguous. See text for details.*

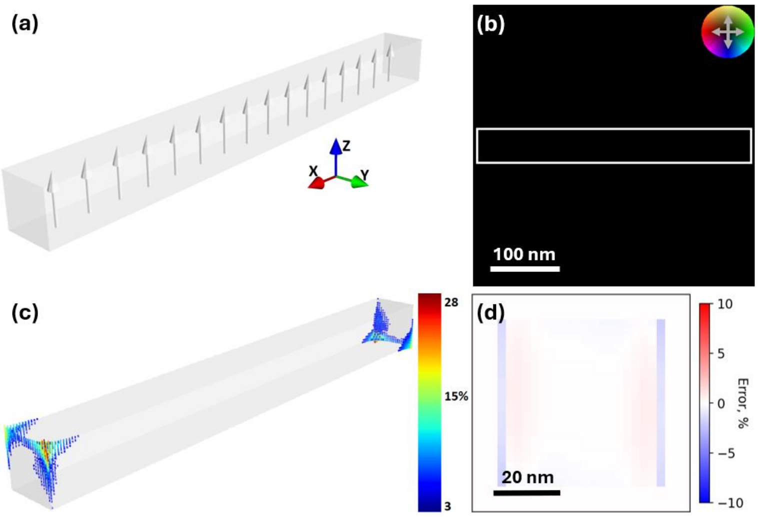


*Fig. S3. **Reconstruction of a simulated nanowire magnetised along the z-axis.** (a) Model of a 400-nm-long, 50 nm x 50 nm nanowire, showing the sample geometry and the $\vec{M}$ direction. (b) Phase contour map at 0° tilt, coloured to show the direction of the projected in-plane $\vec{B}$ field (inset), displayed as $sin(12\varphi_{mag})$. The sample outline is marked in white. (c) Reconstruction with the $\vec{M}$ vectors scaled and coloured to show the magnitudes of errors greater than 3%. (d) Average $\vec{M}$ magnitude error in a cross-section, demonstrating over and under estimates of below 2%. The greatest errors are at the corners of the nanowire, where the separation of $\vec{M}$ and $\vec{H}$ is ambiguous. See text for details.*

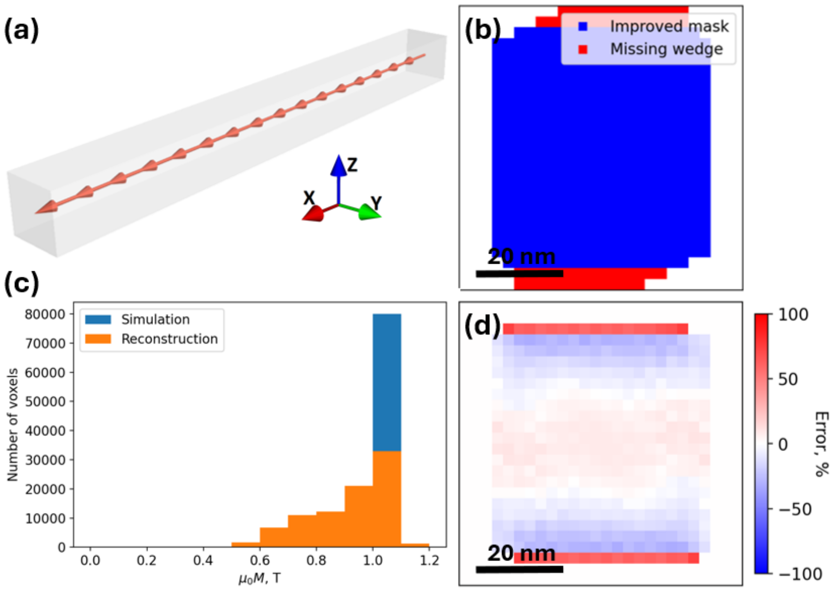


*Fig. S4. **Reconstruction of a simulated nanowire with incomplete missing wedge correction.** (a) Model of a 400-nm-long, 50 nm x 50 nm nanowire, showing the sample geometry and the $\vec{M}$ direction. (b) Reconstructed geometrical model, showing the effect of the missing wedge a in cross-section. (c) Reconstructed $\vec{M}$ magnitude distribution if the missing wedge is not corrected fully. (d) Average $\vec{M}$ magnitude error in a cross-section, showing false values assigned to vacuum and a reduced signal in voxels close to the false region. The surface voxels are incorrect if there are errors when generating the geometrical model. The reconstruction has a mean value of $\mu_0|\vec{M}|$ of 0.92 T and a standard deviation of 0.14 T.*

## S2. Reconstruction of simulated null spaces

Information can be lost at two stages when simulating phase images from a given magnetisation configuration ($\vec{M}$): first when projecting $\vec{M}$ and second when convolving the projected distribution of $\vec{M}$ with a kernel to obtain the corresponding phase [2, 3]. As described in [2], information loss from projection can be avoided by using two complete tilt series. However, information loss during phase calculation is unavoidable, as certain distributions of $\vec{M}$ correspond to eigenstates of a null space and can be added to any reconstruction without changing the corresponding phase images. As null space eigenstates cannot be recovered using MBIR unless appropriate regularising terms are used, null spaces can show $\vec{M} \approx 0$ when they are reconstructed. In practice, null space eigenstates are only known to exist in some ferromagnetic nanostructures, such as fully divergent configurations [2] and Néel-type magnetic domain walls [4]. Here, several such configurations are simulated and compared to a simulation performed for an L-shaped nanowire structure. The effect of projection-based information loss is illustrated in Fig. S5, which shows simulations of magnetic phase images for nanowires that have vortex-type magnetic domain walls at their centres. The nanowires have a diameter of 100 nm, an aspect ratio of 10:1 and $\mu_0|\vec{M}| = 1$ T. The phase images shown in Fig. S5b3 and Fig. S5c3 are indistinguishable if the phase measurements have more than 0.1 % noise, even though they correspond to different configurations of $\vec{M}$. The sample must be tilted, as shown in Fig. S5a, to enable successful reconstruction. In the null space simulations shown below, complete tilt series are simulated to avoid information loss from projection, so that any information loss during reconstruction can be attributed only to phase calculation.

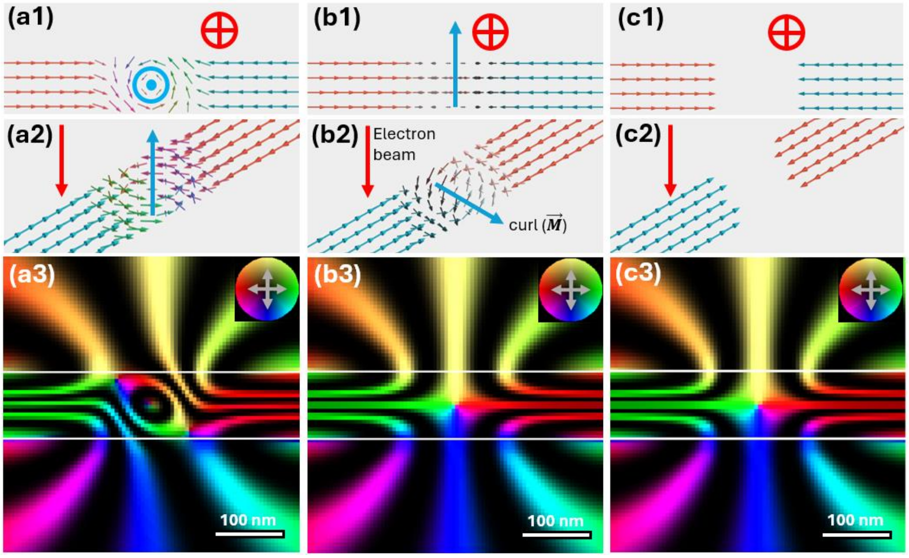


***Fig. S5. Simulated magnetic phase images of non-unique signals in vector field projections.*** *(a1), (b1), (c1) Projections of magnetisation ($\vec{M}$) in the electron beam direction. (a2), (b2), (c3) Isometric projections of $\vec{M}$. The red arrows show the direction of the electron beam. The blue arrows show the direction of $curl(\vec{M})$ at the core of a vortex-type magnetic domain wall. (a3), (b3), (c3) Corresponding magnetic phase contour images, displayed as $cos(5\varphi_{mag})$, coloured to show the direction of the projected in-plane $\vec{B}$ field (inset). The magnetic vortex states only affect the electron phase if $curl(\vec{M})$ has a component parallel to the electron beam direction. Therefore, in (a) the magnetic vortex is imaged perfectly, but in (b) the magnetic domain wall introduces no phase shift and is indistinguishable from the non-magnetic material represented in (c). See text for details.*

Whereas an infinitely-long, first-order Halbach cylinder does not create a magnetic signal in the transmission electron microscope in any projection direction [2, 5], this is not the case for a Halbach cylinder of finite length. Fig. S6a shows a simulation of a 40-nm-long, 40-nm-diameter cylinder with $\mu_0|\vec{\boldsymbol{M}}| = 1$ T, in which $\vec{\boldsymbol{M}}$ is oriented radially outwards and has non-zero divergence at all points, as shown in cross-section in Fig. S6b. Phase images were simulated for a 10° tilt increment about two orthogonal 180° tilt axes, including projections along its axis (Fig. S6c) and perpendicular to its axis (Fig. S6d). Although Fig. S6c is expected to show no magnetic phase shift, a slight residual signal is present close to the surface of the cylinder due to the effects of digitisation (*i.e.*, finite pixel size). In Fig. S6d, there would be no signal if the cylinder were infinitely long. However, a phase shift is present because the cylinder has a finite length. The simulated phase images were used to reconstruct $\vec{\boldsymbol{M}}$ and compared to the input magnetisation distribution. Fig. S7a and S7b show the reconstructed distributions of $\vec{\boldsymbol{M}}$ in cross-section at the surface of the cylinder. The magnitude of $\vec{\boldsymbol{M}}$ is up to two times larger than the input, presumably because there is insufficient signal to distinguish between $\vec{\boldsymbol{M}}$ and the demagnetising field $\vec{\boldsymbol{H}}$. Fig. S7c and S7d show the reconstructed cross-section of the null space in the middle of the cylinder, where the magnitude of $\vec{\boldsymbol{M}}$ is 90 % lower than the input. $\vec{\boldsymbol{M}}$ is also rotated towards the direction of magnetic induction. The simulations show that such configurations, in which $\vec{\boldsymbol{M}}$ is divergent at all points, cannot be reconstructed successfully without the use of additional constraints.

Similar null spaces have been observed when imaging Néel-type magnetic domain walls in thin films that exhibit the interfacial Dzyaloshinskii–Moriya interaction [4, 6, 7]. In order to evaluate possible reconstruction errors, a 100 nm x 100 nm x 50 nm film containing a Néel-type magnetic domain wall was simulated, as shown in Fig. S8a and S8b. Phase images were simulated with a 10° tilt increment about two orthogonal 180° axes. A magnetic phase shift from the uniformly-magnetised parts of the film is detected in all of the projections, as shown in Fig. S8c and S8d. The reconstruction is "correct" in the uniformly-magnetised parts of the film. However, some signal is missing at the magnetic domain wall itself. Fig. S9a and S9b show that the surface reconstruction has a 15% error throughout the magnetic domain wall. $\vec{\boldsymbol{M}}$ is also not separated fully from $\vec{\boldsymbol{H}}$ at the corners of the film. Fig. S9c and S9d show the null space inside the film, where 75 % of the signal is lost at the magnetic domain wall. This loss of signal depends on the magnetic domain wall width. The simulations show that only uniform regions around Néel-type magnetic domain walls can be reconstructed quantitatively in thin films without the use of additional constraints. In addition, qualitative measurement of magnetic domain wall orientation would require a large range of tilt angles, in accordance with previous simulations [1].

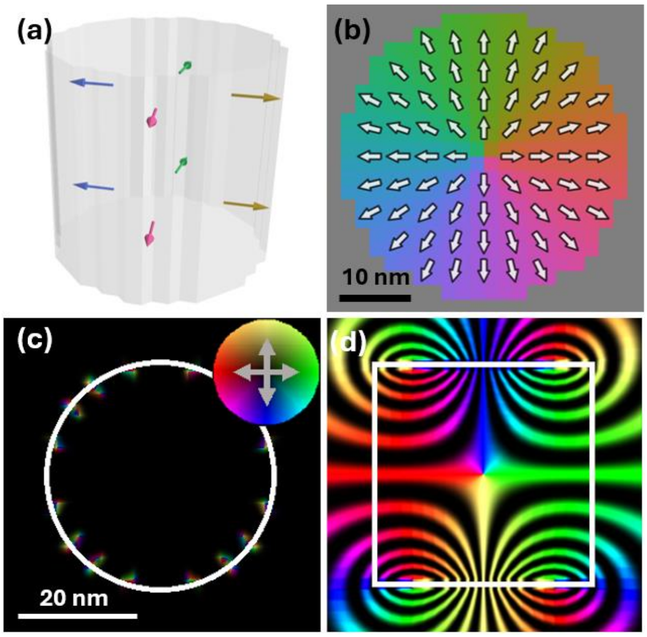


**Fig. S6. Simulated magnetic phase images of a divergent Halbach cylinder.** (a) Model of a 40-nm-long, 40-nm-diameter cylinder showing the sample geometry and the $\vec{M}$ direction. (b) $\vec{M}$ distribution in a cross section of the sample. (c) Phase contour map generated along the axis of the cylinder. (d) Phase contour map generated perpendicular to the axis of the cylinder. The phase contour images are coloured to show the direction of the projected in-plane $\vec{B}$ field (inset), displayed as $cos(200\varphi_{mag})$. The sample outline is marked in white. An infinitely-long Halbach cylinder would not create a magnetic signal in any projection direction. In contrast, the finite version creates a signal in some projection directions.

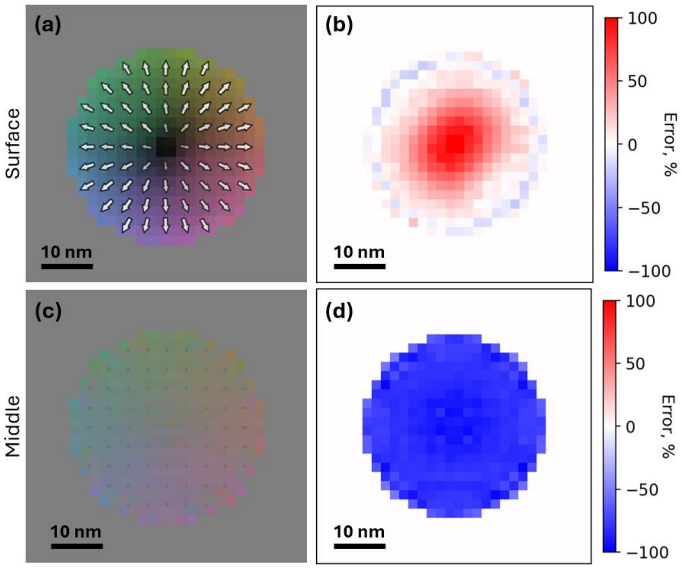


***Fig. S7. Reconstruction of a simulated divergent Halbach cylinder.*** *(a) Reconstructed $\vec{M}$ cross-section at the surface. (b) Magnitude of error at the surface, showing an overestimate of up to 110 %. (c) Reconstructed $\vec{M}$ cross-section in the middle of the cylinder. (d) Magnitude of error in the middle, showing a 90 % loss of signal. The $\vec{M}$ magnitude is greater than it should be at the surface because $\vec{M}$ and $\vec{H}$ were not separated correctly. In the middle of the cylinder, the magnitude is 90 % lower than the ground truth because almost no signal is detected from this region.*

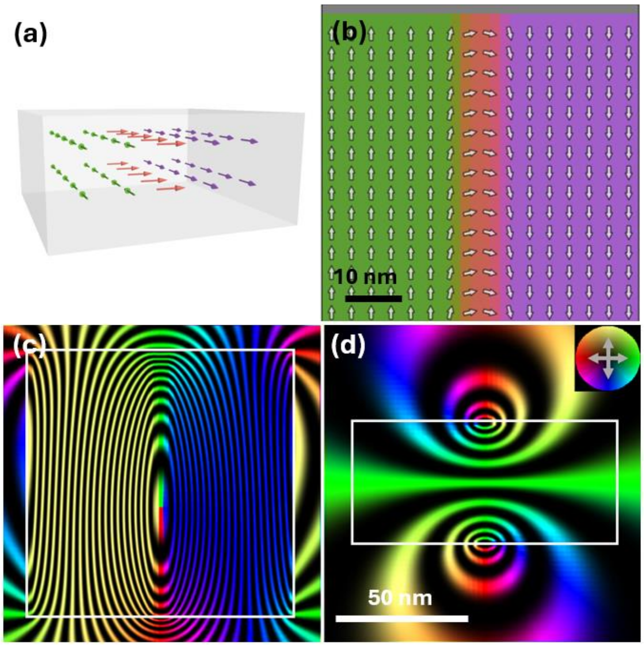


***Fig. S8. Simulated magnetic phase images of a Néel-type magnetic domain wall.*** *(a) Model of 100 nm x 100 nm x 50 nm sample containing a Néel-type magnetic domain wall, showing the sample geometry and the $\vec{M}$ direction. (b) $\vec{M}$ distribution in a slice of the sample close to the edge. (c) Top-down phase contour map. (d) Sideways phase contour map. The magnetic phase contour images are coloured to show the direction of the projected in-plane $\vec{B}$ field (inset), displayed as $cos(40\varphi_{mag})$. The sample outline is marked in white. The signal from the uniformly-magnetised domains is detected, but some of the signal from the magnetic domain wall is lost.*

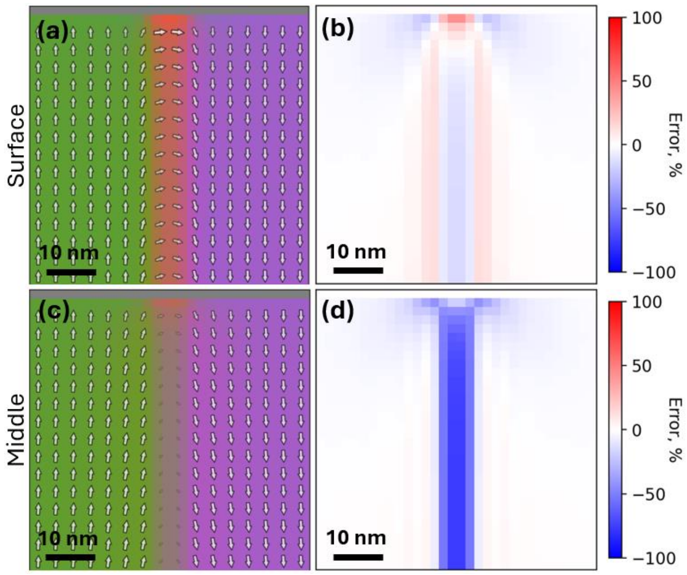


***Fig. S9. Reconstruction of a simulated Néel-type magnetic domain wall.*** *(a) Reconstructed $\vec{M}$ slice at the surface. (b) Vector magnitude error at the surface, showing an overestimate of 50% at the corner of the film and errors of 15% at the magnetic domain wall surface. (c) Reconstructed $\vec{M}$ slice in the middle of the film. (d) Magnitude of error in the middle of the film, showing a 75 % loss of signal at the magnetic domain wall. The surface of the Néel-type magnetic domain wall can be reconstructed, but there is a null space in the centre. See text for details.*

Néel-type magnetic domain walls may also be present in nanowire structures. The magnetic domain wall width in cobalt nanowires has been observed to be ~100 nm [8] and the rotation of $\vec{\boldsymbol{M}}$ in the wall may be smaller than 180°. A Néel-type magnetic domain wall was simulated in an L-shaped, 600-nm-long, 100-nm-wide, square-cross-section nanowire, as shown in Fig. S10a and S10b. Phase images were simulated with a 10° tilt increment about two orthogonal 180° axes, as shown in Fig. S10c and S10d. The reconstruction in Fig. S11 shows that the full volume of the reconstruction acquires a 1 % error as a result of the difficulty of separating $\vec{\boldsymbol{M}}$ and $\vec{\boldsymbol{H}}$. Fig. S11d shows that up to 5 % of the signal is lost in the middle of the magnetic domain wall, suggesting that null space effects in such nanowires can be smaller than those in extended thin films.

With regard to the results described in the main text, simulations have previously been used to show that magnetic vortex states do not result in null spaces if they are imaged close to the direction of the curl of the magnetic vortex [1]. In the absence of a significant null space contribution, any errors associated with the separation of $\vec{\boldsymbol{M}}$ and $\vec{\boldsymbol{H}}$ should be comparable to the ~2% random error in the reconstruction discussed in the main text.

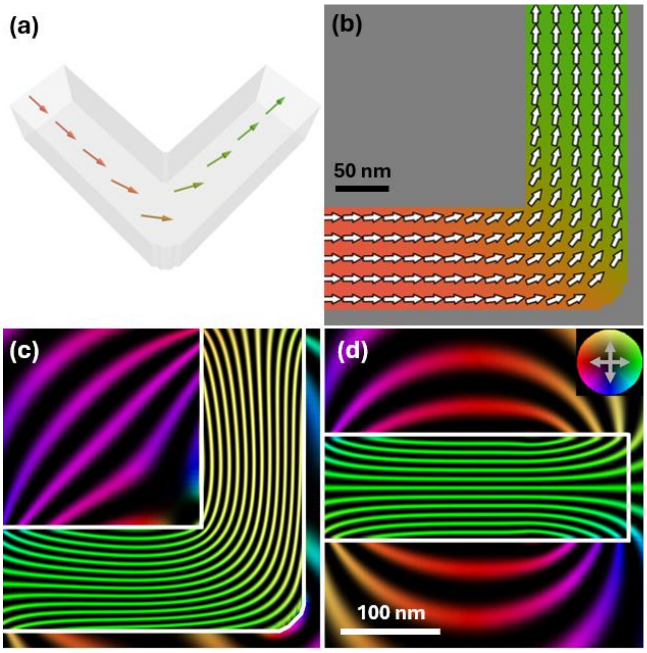


***Fig. S10. Simulated magnetic phase images of a nanowire with a Néel-type magnetic domain wall.*** *(a) Model of 100 nm x 100 nm cross-section nanowire with a Néel-type magnetic domain wall, showing the sample geometry and the* $\vec{M}$ *direction. (b)* $\vec{M}$ *distribution in a slice of the sample. (c) Top-down phase contour map. (d) Sideways phase contour map. The magnetic phase contour images are coloured to show the direction of the projected in-plane* $\vec{B}$ *field (inset), displayed as* $cos(6\varphi_{mag})$*. The sample outline is marked in white. The magnetic phase shift is detected from all parts of the nanowire structure.*

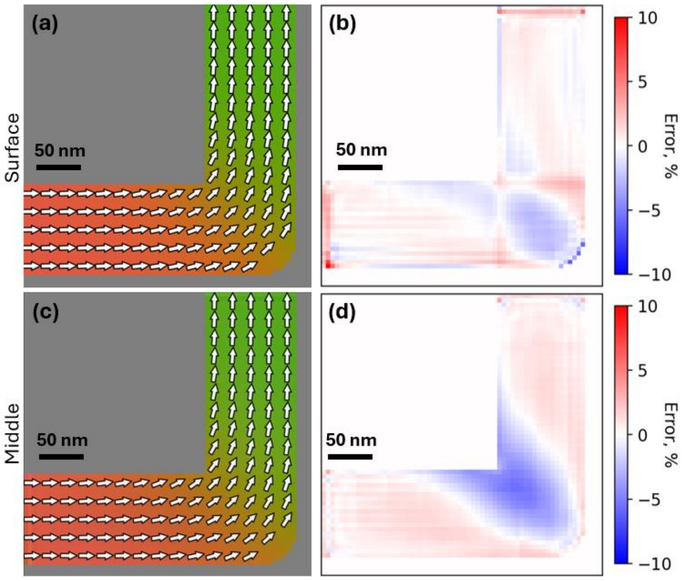


***Fig. S11. Reconstruction of a simulated nanowire with a Néel-type magnetic domain wall.*** *(a) Reconstructed* $\vec{M}$ *slice at the surface. (b) Vector magnitude error at the surface, showing 1 % errors throughout. (c) Reconstructed* $\vec{M}$ *slice in the middle of the film. (d) Magnitude of error in the middle, showing a 5 % loss of signal at the centre of the magnetic domain wall. In a nanowire, the Néel-type magnetic domain wall null space is reduced. See text for details.*

## S3. Software

The primary scientific software packages used in this study, their roles in the workflow (Fig. S12), their repositories and relevant accompanying publications (if available) are listed here:

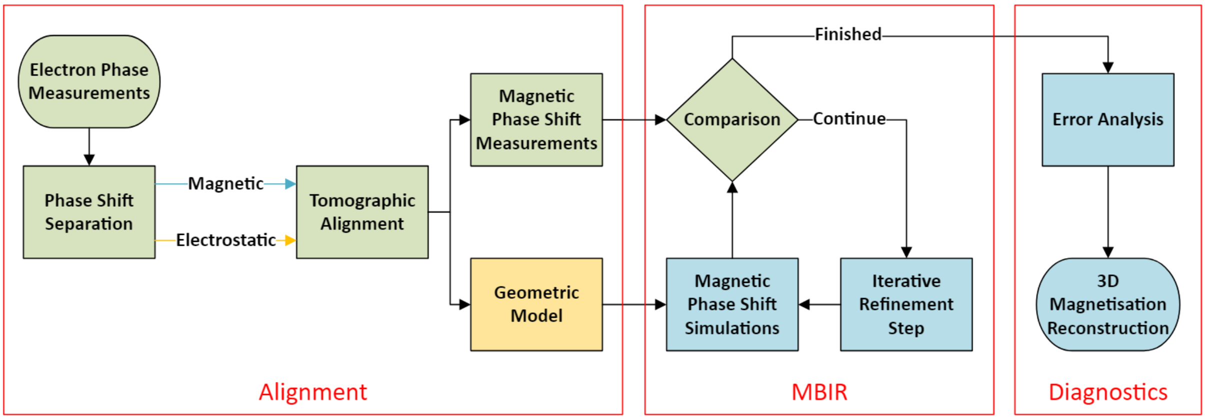


***Fig. S12. Workflow for 3D magnetisation reconstruction.*** *The red boxes indicate the primary processing steps: alignment, reconstruction using MBIR, and diagnostics. Datasets are processed to generate both a geometrical mask that defines where the magnetic material is located and a series of magnetic phase shift measurements corresponding to* $\vec{B}$ *field projections. At each iteration, a distribution of* $\vec{M}$ *is generated, and then its magnetic phase shift is simulated and compared to the measurements. The iterations are repeated until an optimal* $\vec{M}$ *is found. Optimal estimation diagnostics are performed to assess random and systematic errors in the reconstruction. The steps are shaded to indicate the data type that is being processed: two-dimensional phase images (green), 3D magnetic vector fields (blue) and a 3D electrostatic scalar field (yellow).*

- **MBIR-TEM**. MBIR-based magnetisation reconstruction package guiding the workflow [9].
  Repository: https://github.com/AurysSilinga/MBIR-TEM
- **F3ast**. FEBID modelling package used for sample fabrication with CAD [10].
  Repository: https://github.com/skoricius/f3ast
- **Gatan DigitalMicrograph** with **Holoview** and **HoloWorks** plugins. Hologram-to-phase reconstruction [11][12].
  Repository: http://www.dmscripting.com
- **Hyperspy**. Interface between DigitalMicrograph and Python, with interactive image manipulation in Python [13].
  Repository: https://hyperspy.org/
- **scikit-image**. Canny edge detection and image manipulation for phase shift separation [14].
  Repository: https://scikit-image.org/
- **fpd**. Image feature matching for phase shift separation and RANSAC-algorithm-based background removal for tomographic alignment [15].
  Repository: https://gitlab.com/fpdpy/fpd
- **Scipy**. Error function minimisation for tomographic alignment [16].
  Repository: https://scipy.org/
- **jutil**. Conjugate gradient minimisation for MBIR.
  Repository: https://jugit.fz-juelich.de/j.ungermann/jutil
- **Pyramid**. MBIR simulations [17].
  Repository: https://iffgit.fz-juelich.de/empyre/empyre/-/tree/pyramid-master

## S4. Phase reconstruction using off-axis electron holography

Off-axis electron holography is a transmission electron microscopy (TEM) technique that can be used to measure the phase shift of an electron wavefront. The technique was employed to acquire the tomographic series of phase images described in the main text. Fig. S13 shows an electron-optical ray diagram, in which the electron beam is split into an object wave and a reference wave, which interfere and form a hologram on the detector. Fig. S14 shows an example of the reconstruction of the relative phase shift between the object and reference wave from a hologram. For accurate reconstruction, there should not be any electromagnetic fields in the reference wave. In practice, long-range fields from the sample and residual fields from the TEM components can perturb the reference wave. The residual fields from the TEM components can be measured and corrected by acquiring a reference hologram in free space. Fig. S15 shows an example of combining two reconstructed phase shift images to separate the electrostatic and magnetic contributions to the phase shift. The processing steps were performed using a combination of Gatan Digital Micrograph and Python scripts listed in section S3.

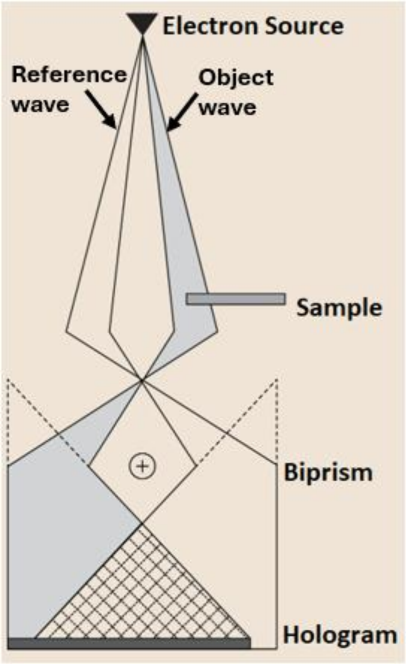


***Fig. S13.*** *Ray diagram for the TEM mode of off-axis electron holography. An electron biprism is used to split the electron beam into two waves, which interfere and form a hologram on the detector. Electromagnetic fields in the sample affect the spacing of the interference fringes in the hologram. Reproduced from [18].*

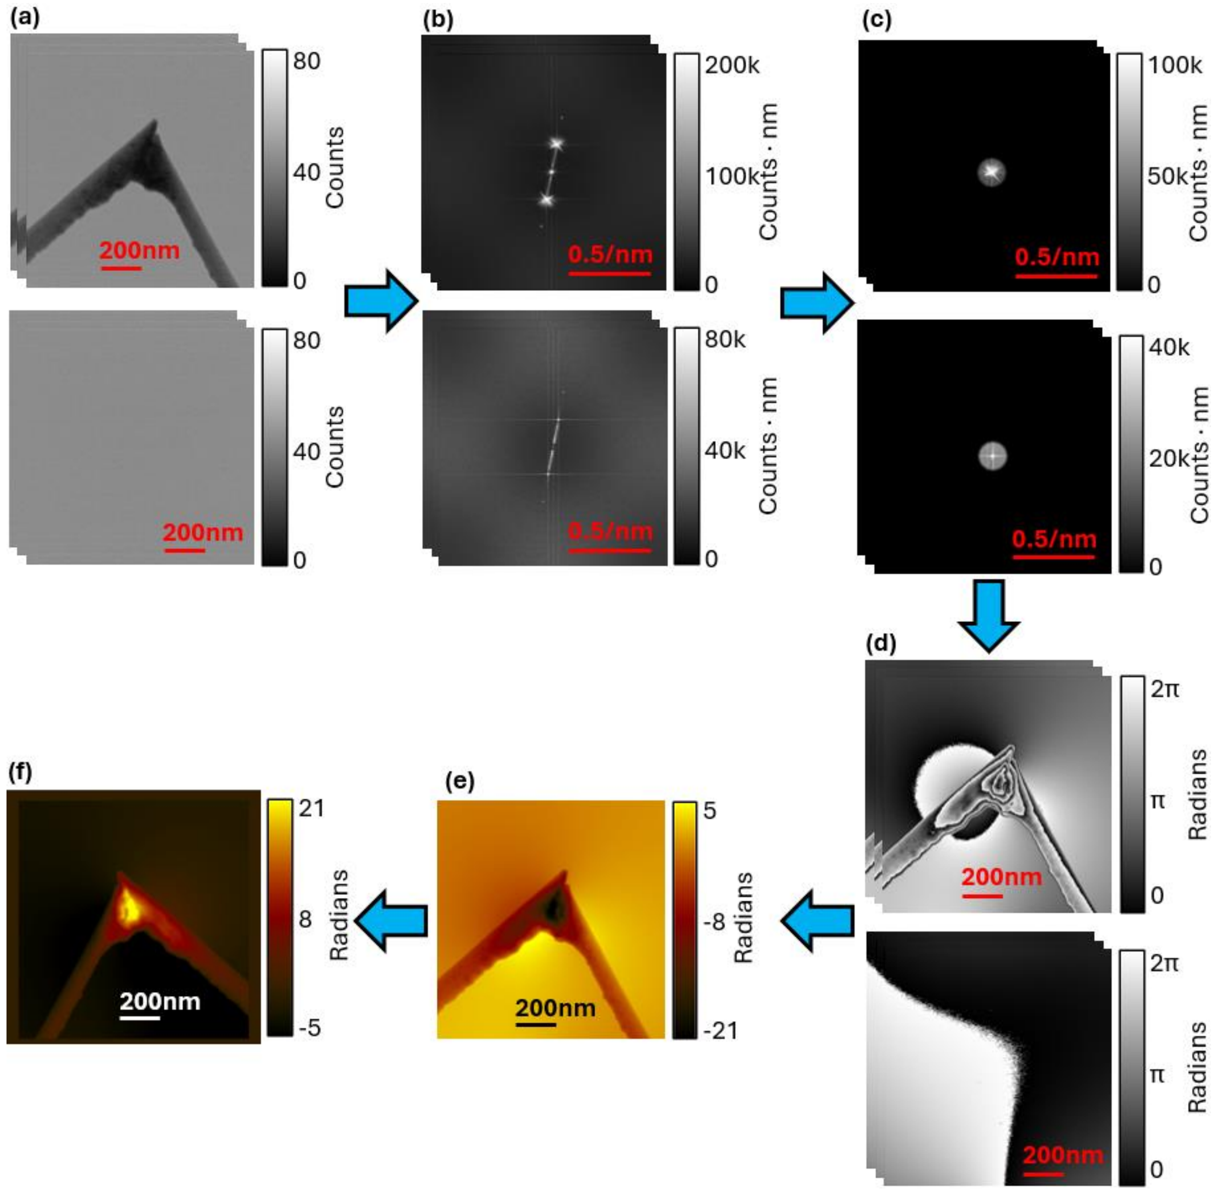


***Fig. S14.*** *Steps involved in hologram-to-phase reconstruction. (a) Off-axis electron hologram of the sample (top) and a reference hologram of free space (bottom). Five holograms were acquired with 2 s exposure times each. The holographic interference fringe spacing is below 3 nm. (b) Fast Fourier transforms (FFTs) of the holograms, displayed as the magnitudes of the complex arrays. The sidebands are centred on a spatial frequency of ~0.35 rad/nm. (c) The streaks are masked to reduce the effects of Fresnel fringes at the edges of the biprism wire and a virtual aperture is applied to select one sideband. (d) An inverse FFT is applied to the masked image, resulting in a complex real-space image. The phase of the complex images, which corresponds to the phase difference between the object and reference waves, is shown. The difference between the minimum and maximum values of the vacuum measurement is ~5 radians. (e) The phase images are "unwrapped" to remove 2π phase discontinuities and averaged to reduce measurement noise. The vacuum perturbation is then subtracted. (f) In order to ensure consistency, the image is rotated such that the tomographic tilt axis is less than 15° from the horizontal. The sign of the image is also reversed, such that the electrostatic mean inner potential is positive (following the convention generally used in electron microscopy).*

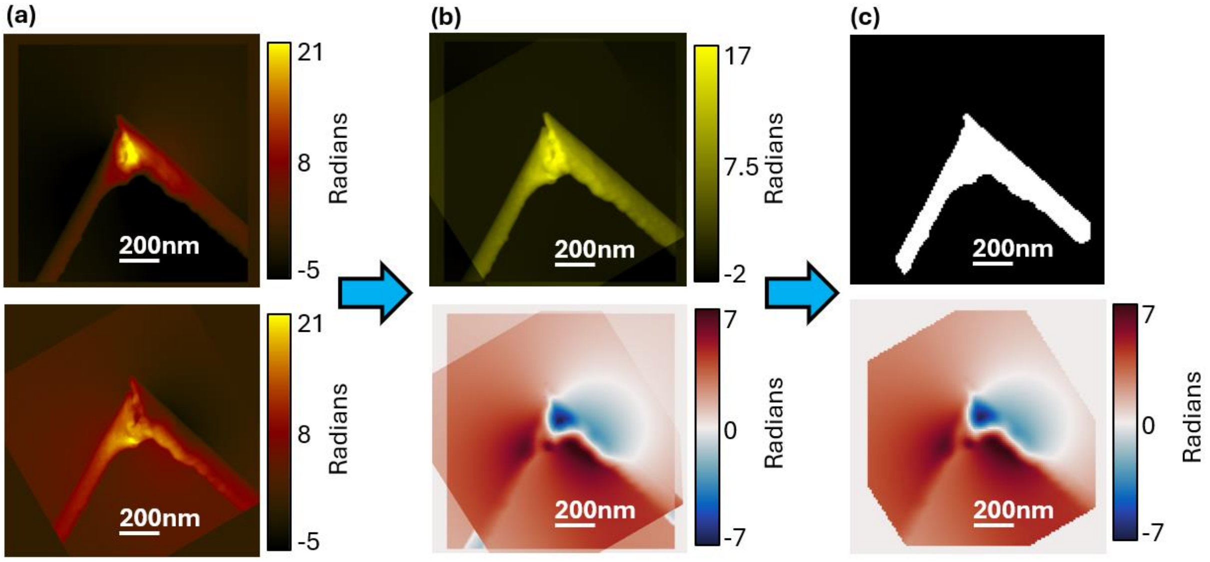


***Fig. S15.*** *Separation of electrostatic and magnetic contributions to the electron phase shift. (a) Total phase shift images recorded at −3.7° tilt (top) and 176° tilt (bottom). Both images have been reconstructed following the procedure described in Fig. S14 and aligned with sub-pixel precision using the edge detection method described in the main text. (b) The images in (a) are added and divided by two to calculate the half-sum image (top) and subtracted and divided by two to calculate the half-difference image (bottom). The half-sum image is the electrostatic phase shift, which is proportional to the mean-inner-potential and the specimen thickness. The half-difference image is the magnetic phase shift, which is related to the projection of the magnetic induction in the electron beam direction. (c) Both images are further processed before reconstruction with MBIR. A threshold is applied to the electrostatic phase shift (top) to define the location of the sample. Gaussian smoothing is applied to the magnetic phase shift image (bottom) to reduce noise, the image is rebinned from 0.65 nm/ pixel size to 10.4 nm/ pixel to reduce computational time and the overlap region of images in (a) is identified to set the confidence mask. The use of smaller pixel sizes increases computation time and does not improve the resolution of the final reconstruction, which is limited by factors that include tomographic alignment in the present work.*

## S5. MBIR cost function minimisation

During MBIR, a forward model $F$ is used to convert a magnetisation distribution $\vec{\boldsymbol{M}}$ in a 3D volume into a tilt series of simulated magnetic phase images [19]:

$$\varphi_{1,calc}, \dots, \varphi_{n,calc} = F(\vec{\boldsymbol{M}}) \,. \tag{S1}$$

Conversely, a magnetisation distribution that satisfies the magnetic phase measurements can be determined by minimising a cost function of the form

$$C = \sum_i \left(\varphi_{i,meas} - \varphi_{i,calc}(\vec{\boldsymbol{M}})\right)^2 + \lambda_1(\nabla\vec{\boldsymbol{M}} \cdot \nabla\vec{\boldsymbol{M}}) + \lambda_2 \mathrm{var}(|\vec{\boldsymbol{M}}|)\,, \tag{S2}$$

where $C$ is the cost, $\vec{\boldsymbol{M}}$ is the magnetisation vector field, $\varphi$ are the phase images, $\lambda$ are the regulariser weights, $\nabla$ is the gradient operator and 'var' is the variance operator. In order to account for multiple possible solutions for $\vec{\boldsymbol{M}}$, regularising terms are used, for example to favour a solution that exhibits a low gradient or a small variance in the magnitude of the magnetisation. A low gradient favours ferromagnetic order, while a small variance favours a sample that contains similar materials. The cost function is minimised by using a preconditioned conjugate gradient method [20] to find the optimal solution for the magnetisation.

In the phase object approximation, the forward model for phase image calculation can be written in the form [19]

$$\varphi_{mag}(x, y) = \frac{-\mu_0}{2\Phi_0} \iint \frac{(y - y')\, M_x(x,y) - (x-x')\, M_y(x,y)}{(x-x')^2 + (y-y')^2}\, \mathrm{d}x'\mathrm{d}y' \,, \tag{S3}$$

where $\Phi_0$ is a magnetic flux quantum and $M_x$ and $M_y$ are projected magnetisation values in the *x* and *y* directions, respectively. The use of a geometrical model to describe the sample reduces the number of magnetisation voxels used in the calculation. The convolution can be optimised by implementing it in reciprocal space. Instead of evaluating the convolution at each phase image pixel, each projected magnetisation pixel can be assumed to be a magnetised disk, for which the phase shift can be described analytically. All of the phase image pixels can then be calculated simultaneously by convolving the phase contribution from a single magnetised disk with all of the positions at which magnetic moments are located. This approach improves the scaling of the execution time from $O(\mathrm{N}^4)$ to $O\big(N^2 log(N)\big)$, where $N$ is the number of magnetisation voxels.

## S6. Correlation between $\overrightarrow{M}$ and atomic composition

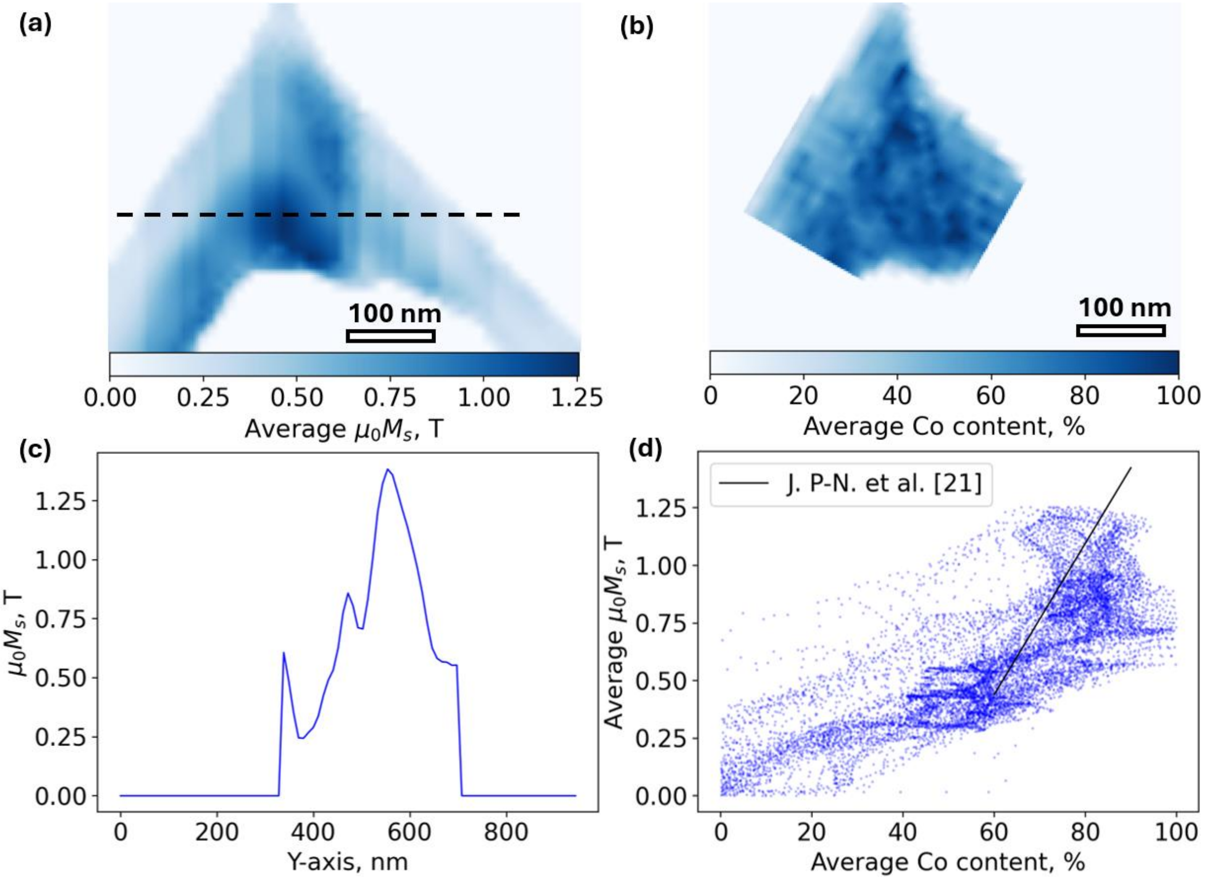


***Fig. S16.*** *Correlation between the experimental reconstruction of $\overrightarrow{M}$ and the atomic composition measured using electron energy-loss spectroscopy (EELS). (a) Average value of $\mu_0|\overrightarrow{M}|$ projected at 0° tilt. (b) EELS measurement of the projected Co atomic content at 0° tilt. The image was interpolated and rotated to match the scale and number of pixels in (a). (c) Line trace showing $\mu_0|\overrightarrow{M}|$ for one line of voxels in the reconstruction. The z-coordinate of the line trace is in the centre of the reconstructed volume, while the x-coordinate position and y-coordinate extent correspond to the dashed line in image (a). (d) Correlation between overlapping pixels in images (a) and (b). A calibration between atomic Co content and $\overrightarrow{B}$ in high-aspect-ratio FEBID nanowires [21] is shown in black. (c) shows an artefact on the left side, which is attributed to surface digitisation and is believed to result from tomographic misalignment. If the geometrical model were too small, then artefacts on both sides would be expected. The majority of the data points in (d) are close to predictions from previous work, with similar amounts of under- and over-estimates attributed to artefacts in the reconstruction or alignment of images (a) and (b). Points showing non-zero $M_s$ when the Co content is below 40% do not follow the expected trend and are believed to correspond to areas where ferromagnetic and paramagnetic material overlap in projection, or to regions where inaccurate values are assigned to vacuum due to the limited spatial resolution. Overall, most of the reconstructed data points agree with previous work, although some artefacts are present.*

## References


[1] Caron, J., 2018. Magnetisation reconstruction in three dimensions, in: Model-based reconstruction of magnetisation distributions in nanostructures from electron optical phase images, FZJ-2018-05288. Ph.D. thesis, Forschungszentrum Jülich GmbH Zentralbibliothek, Verlag, Jülich, pp. 119–140. http://hdl.handle.net/2128/19740

[2] Caron, J., 2018. Reconstructibility and null spaces, in: Model-based reconstruction of magnetisation distributions in nanostructures from electron optical phase images, FZJ-2018-05288. Ph.D. thesis, Forschungszentrum Jülich GmbH Zentralbibliothek, Verlag, Jülich, pp. 74–82. http://hdl.handle.net/2128/19740

[3] Mansuripur, M., 1991. Computation of electron diffraction patterns in Lorentz electron microscopy of thin magnetic films. J. Appl. Phys. 69, 2455–2464. https://doi.org/10.1063/1.348682

[4] Benitez, M.J., Hrabec, A., Mihai, A.P., Moore, T.A., Burnell, G., McGrouther, D., Marrows, C.H., McVitie, S., 2015. Magnetic microscopy and topological stability of homochiral Néel domain walls in a Pt/Co/AlOx trilayer. Nat. Commun. 6, 8957. https://doi.org/10.1038/ncomms9957

[5] Halbach, K., 1980. Design of permanent multipole magnets with oriented rare earth cobalt material. Nucl. Instrum. Methods 169, 1–10. https://doi.org/10.1016/0029-554X(80)90094-4

[6] McVitie, S., Hughes, S., Fallon, K., McFadzean, S., McGrouther, D., Krajnak, M., Legrand, W., Maccariello, D., Collin, S., Garcia, K., Reyren, N., Cros, V., Fert, A., Zeissler, K., Marrows, C.H., 2018. A transmission electron microscope study of Néel skyrmion magnetic textures in multilayer thin film systems with large interfacial chiral interaction. Sci. Rep. 8, 5703. https://doi.org/10.1038/s41598-018-23799-0

[7] Jiang, W., 2019. Quantifying chiral exchange interaction for Néel-type skyrmions via Lorentz transmission electron microscopy. Phys. Rev. B 99. https://doi.org/10.1103/PhysRevB.99.104402

[8] Donnelly, C., Hierro-Rodríguez, A., Abert, C., Witte, K., Skoric, L., Sanz-Hernández, D., Finizio, S., Meng, F., McVitie, S., Raabe, J., Suess, D., Cowburn, R., Fernández-Pacheco, A., 2022. Complex free-space magnetic field textures induced by three-dimensional magnetic nanostructures. Nat. Nanotechnol. 17, 136–142. https://doi.org/10.1038/s41565-021-01027-7

[9] Silinga, A., Kovács, A., McVitie, S., Dunin-Borkowski, R.E., Fallon, K., Almeida, T.P., 2024. 3-Model-Based Iterative Reconstruction of Three-Dimensional Magnetisation in a Nanowire Structure Using Electron Holographic Vector Field Tomography. Preprint. https://doi.org/10.48550/arXiv.2411.15323

[10] Skoric, L., Sanz-Hernández, D., Meng, F., Donnelly, C., Merino-Aceituno, S., Fernández-Pacheco, A., 2020. Layer-by-Layer Growth of Complex-Shaped Three-Dimensional Nanostructures with Focused Electron Beams. Nano Lett. 20, 184–191. https://doi.org/10.1021/acs.nanolett.9b03565

[11] Boureau, V., McLeod, R., Mayall, B., Cooper, D., 2018. Off-axis electron holography combining summation of hologram series with double-exposure phase-shifting: Theory and application. Ultramicroscopy 193, 52–63. https://doi.org/10.1016/j.ultramic.2018.06.004

[12] Mitchell, D.R.G., Schaffer, B., 2005. Scripting-customised microscopy tools for Digital Micrograph™. Ultramicroscopy 103, 319–332. https://doi.org/10.1016/j.ultramic.2005.02.003

[13] Peña, F. de la, Prestat, E., Fauske, V.T., Burdet, P., Jokubauskas, P., Nord, M., Ostasevicius, T., MacArthur, K.E., Sarahan, M., Johnstone, D.N., Taillon, J., Lähnemann, J., Migunov, V., Eljarrat, A., Caron, J., Aarholt, T., Mazzucco, S., Walls, M., Slater, T., Winkler, F., pquinn-dls, Martineau, B., Donval, G., McLeod, R., Hoglund, E.R., Alxneit, I., Lundeby, D., Henninen, T., Zagonel, L.F., Garmannslund, A., 2019. hyperspy/hyperspy: HyperSpy v1.5.2. https://doi.org/10.5281/zenodo.3396791

[14] Walt, S. van der, Schönberger, J.L., Nunez-Iglesias, J., Boulogne, F., Warner, J.D., Yager, N., Gouillart, E., Yu, T., 2014. scikit-image: image processing in Python. PeerJ 2:e453. https://doi.org/10.7717/peerj.453

[15] Paterson, G.W., Webster, R.W.H., Ross, A., Paton, K.A., Macgregor, T.A., McGrouther, D., MacLaren, I., Nord, M., 2020. Fast Pixelated Detectors in Scanning Transmission Electron Microscopy. Part II: Post-Acquisition Data Processing, Visualization, and Structural Characterization. Microsc. Microanal. 26, 944–963. https://doi.org/10.1017/S1431927620024307

[16] Virtanen, P., Gommers, R., Oliphant, T.E., Haberland, M., Reddy, T., Cournapeau, D., Burovski, E., Peterson, P., Weckesser, W., Bright, J., van der Walt, S.J., Brett, M., Wilson, J., Millman, K.J., Mayorov, N., Nelson, A.R.J., Jones, E., Kern, R., Larson, E., Carey, C.J., Polat, İ., Feng, Y., Moore, E.W., VanderPlas, J., Laxalde, D., Perktold, J., Cimrman, R., Henriksen, I., Quintero, E.A., Harris, C.R., Archibald, A.M., Ribeiro, A.H., Pedregosa, F., van Mulbregt, P., 2020. SciPy 1.0: fundamental algorithms for scientific computing in Python. Nat. Methods. 17, 261–272. https://doi.org/10.1038/s41592-019-0686-2

[17] Caron, J., 2018. Model-based reconstruction of magnetisation distributions in nanostructures from electron optical phase images, FZJ-2018-05288. Ph.D. thesis, Forschungszentrum Jülich GmbH Zentralbibliothek, Verlag. http://hdl.handle.net/2128/19740

[18] Dunin-Borkowski, R.E., Kovács, A., Kasama, T., McCartney, M.R., Smith, D.J., 2019. Electron Holography, in: Hawkes, P.W., Spence, J.C.H. (Eds.), Springer Handbook of Microscopy. Springer International Publishing, Cham, pp. 767–818. https://doi.org/10.1007/978-3-030-00069-1_16

[19] Caron, J., 2018. A forward model for the calculation of the magnetic phase, in: Model-based reconstruction of magnetisation distributions in nanostructures from electron optical phase images, FZJ-2018-05288. Ph.D. thesis, Forschungszentrum Jülich GmbH Zentralbibliothek, Verlag, Jülich, pp. 21–57. http://hdl.handle.net/2128/19740

[20] Caron, J., 2018. Solving the inverse problem of magnetisation retrieval, in: Model-based reconstruction of magnetisation distributions in nanostructures from electron optical phase images, FZJ-2018-05288. Ph.D. thesis, Forschungszentrum Jülich GmbH Zentralbibliothek, Verlag, Jülich, pp. 59–82. http://hdl.handle.net/2128/19740

[21] Pablo-Navarro, J., Magén, C., de Teresa, J.M., 2018. Purified and Crystalline Three-Dimensional Electron-Beam-Induced Deposits: The Successful Case of Cobalt for High-Performance Magnetic Nanowires. ACS Appl. Nano Mater. 1, 38–46. https://doi.org/10.1021/acsanm.7b00016
